# Supplementary material for: The threshold of semiconductor nanolasers
Source: arXiv:2305.15888 ancillary file (2023-08-31)
Supplement: Supplementary file 1 [file Threshold_Semiconductor_Nanolasers__Supplementary.pdf]

# Supplementary Material for "The threshold of semiconductor nanolasers"

Marco Saldutti, Yi Yu, and Jesper Mørk\*

DTU Electro, Technical University of Denmark, DK-2800 Kgs. Lyngby, Denmark and  
NanoPhoton - Center for Nanophotonics, Technical University of Denmark, DK-2800 Kgs. Lyngby, Denmark

(Dated: August 31, 2023)

## I. SPONTANEOUS EMISSION RATE PER EMITTER

In this section, we formally derive the spontaneous emission rate per emitter,  $\gamma_r$ . Importantly, we discuss the mode volume entering the expression of  $\gamma_r$  in the case of a single emitter and the more general situation of an extended semiconductor active medium. We restrict the analysis to the weak-coupling regime [1, 2], where rate equation descriptions apply.

From Fermi's golden rule, the spontaneous emission rate of an emitter embedded in an optical cavity is proportional to the local **photonic density of states** (LDOS) [3]. This represents the density of optical modes, per unit frequency and unit volume, at the position of the emitter. The calculation of the LDOS is a subtle issue, which essentially amounts to computing the so-called *quasi-normal* modes (QNMs) [4].

Also known as leaky modes [5], QNMs are solutions of time-harmonic, source-free Maxwell's equations with radiation boundary conditions. Their frequencies are complex, with the imaginary part being the damping rate of the mode. Importantly, the boundary conditions ensure that energy leaks away from the resonator, but they also imply that the field distributions diverge in space at sufficiently large distances from the cavity. This divergence raises the crucial question of the QNMs normalization [6–8], which is at the core of a rigorous definition of the optical mode volume [9–12].

### A. Single emitter

We start by considering a single emitter, e.g. a quantum dot (QD), placed inside the cavity at the position  $\mathbf{r}_e$  and described as an ideal two-level system.

For an ideal, lossless cavity, Maxwell's equations may be reduced to an *hermitian* eigenvalue problem [13], implying that the eigenfrequencies are real and the eigenmodes constitute a complete orthonormal basis - the so-called *normal* modes. In the presence of losses, the eigenvalue problem becomes non-hermitian [14]. However, if the losses are small, the field distributions and the real part of the eigenfrequencies are unchanged to

the first order. At the same time, the resonances are broadened with a Lorentzian lineshape.

Under these assumptions, the LDOS reads [11]

$$\rho_{\text{opt}}(\mathbf{r}_e, \omega) = \sum_m \frac{1}{V_{\text{opt},m}(\mathbf{r}_e)} \left[ \frac{1}{\pi} \frac{\gamma_{c_m}/2}{(\omega - \omega_{c_m})^2 + (\gamma_{c_m}/2)^2} \right] \quad (1)$$

where the summation is over the modes of the cavity. The resonance frequency and damping rate of the  $m$ -th mode are  $\omega_{c_m}$  and  $\gamma_{c_m}/2$ , respectively. The mode volume,  $V_{\text{opt},m}(\mathbf{r}_e)$ , is defined by

$$\frac{1}{V_{\text{opt},m}(\mathbf{r}_e)} = \frac{\epsilon_0 n^2(\mathbf{r}_e) |\hat{\mathbf{d}}_e \cdot \mathbf{E}_m(\mathbf{r}_e)|^2}{\int_V \epsilon_0 n^2(\mathbf{r}) |\mathbf{E}_m(\mathbf{r})|^2 d^3\mathbf{r}} \quad (2)$$

Here,  $\mathbf{E}_m$  is the electric field of the  $m$ -th mode and  $n(\mathbf{r}_e)$  is the refractive index at the position of the emitter. The emitter dipole moment is denoted by  $\mathbf{d}_e = d_e \hat{\mathbf{d}}_e$ , with  $\hat{\mathbf{d}}_e$  being the unit vector which represents the orientation of the dipole. The integration volume,  $V$ , deserves some comments.

In the far field of the resonator, the amplitude of the  $m$ -th mode grows like  $\exp[\gamma_{c_m} r/(2c)]/r$  [9], with  $r = |\mathbf{r}|$  being the amplitude of the position vector and  $c$  being the light speed. Therefore, the integral at the denominator of Eq. 2 diverges as the integration volume tends to infinity. However, the exponential growth of the mode starts only being effective at a distance  $r \approx Q_m \lambda_m/\pi$  from the cavity, with  $Q_m = \omega_{c_m}/\gamma_{c_m}$  being the quality factor of the mode and  $\lambda_m$  the resonant wavelength. Consequently, if the quality factor is high enough, the mode volume can be computed, for all practical purposes, by using Eq. 2. The integration volume can be truncated more or less arbitrarily if enclosing the physical volume of the cavity with a margin of a few wavelengths. The approach is reasonable for the lasing mode of nanolasers with extreme dielectric confinement, but not, e.g., for plasmonic nanolasers [15, 16], where substantial ohmic losses strongly limit the quality factor. In this case, leakage cannot be viewed as a small perturbation and generalized versions [9–12] of Eq. 1 and Eq. 2 should be employed.

We are interested in the spontaneous emission rate into the lasing mode. Hence, we must isolate this mode from Eq. 1. By taking into account the homogeneous broadening of the emitter, Fermi's Golden rule reads

---

\* Correspondence email address: jesm@dtu.dk

[2]

$$\bar{r}_{\text{sp}_0}(\mathbf{r}_e, E_{21}) = \frac{2\pi}{\hbar^2} d_e^2 \int \frac{\hbar\omega}{2\epsilon_0 n^2(\mathbf{r}_e)} \rho_c(\mathbf{r}_e, \omega) L(\hbar\omega - E_{21}) d\omega \quad (3)$$

Here,  $\rho_c(\mathbf{r}_e, \omega) = \frac{1}{V_{\text{opt}}(\mathbf{r}_e)} \left[ \frac{1}{\pi} \frac{\gamma_c/2}{(\omega - \omega_c)^2 + (\gamma_c/2)^2} \right]$  is the LDOS of the lasing mode (for simplicity, we have dropped the subscript  $m$ ) and

$$L(\hbar\omega - E_{21}) = \frac{1}{\pi} \frac{\hbar\gamma_2/2}{(\hbar\omega - E_{21})^2 + (\hbar\gamma_2/2)^2} \quad (4)$$

is the **homogeneous broadening** lineshape. This lineshape effectively describes the broadening of the emitter transition energy around a central value,  $E_{21}$ , due to various decoherence processes.

In practice, Eq. 3 can be simplified by noting that the term  $\hbar\omega$  under the integral is slowly varying compared to the LDOS. Thus, we may assume  $\hbar\omega \approx \hbar\omega_c$  and bring this term outside of the integral. Then, Eq. 3 becomes

$$\bar{r}_{\text{sp}_0}(\mathbf{r}_e, E_{21}) \approx E_{\text{vf}}^2(\mathbf{r}_e) \bar{r}_{\text{sp}_0}(E_{21}) \quad (5)$$

Here, the square of the vacuum-field amplitude,  $E_{\text{vf}}^2(\mathbf{r}_e)$ , reads

$$E_{\text{vf}}^2(\mathbf{r}_e) = \frac{\hbar\omega_c}{2\epsilon_0 n^2(\mathbf{r}_e) V_{\text{opt}}(\mathbf{r}_e)} \quad (6)$$

The convolution between the homogeneous broadening lineshape and LDOS of the lasing mode gives [1]

$$\bar{r}_{\text{sp}_0}(E_{21}) = \frac{2d_e^2}{\hbar^2} \frac{\frac{\gamma_c + \gamma_2}{2}}{(\omega_c - \frac{E_{21}}{\hbar})^2 + (\frac{\gamma_c + \gamma_2}{2})^2} \quad (7)$$

We consider Eq. 7 in the so-called **good-cavity limit**,  $\gamma_2 \gg \gamma_c$ . This is the relevant scenario for emitters working at room temperature, where the emitter dephasing time is on the order of a few tens of femtoseconds [17]. By further assuming the emitter to be in resonance with the lasing mode, Eq. 5 reduces to

$$\bar{r}_{\text{sp}_0}(\mathbf{r}_e) = \frac{2d_e^2}{\hbar\epsilon_0 n^2(\mathbf{r}_e)} \frac{\omega_c}{\gamma_2} \frac{1}{V_{\text{opt}}(\mathbf{r}_e)} \quad (8)$$

We note that in the opposite limit,  $\gamma_2 \ll \gamma_c$  (bad-cavity limit), we would find the usual expression [2, 18] for the Purcell factor.

## B. Extended active medium

We now consider an extended semiconductor active medium, such as an active region with multiple quantum well (QW) or QD layers.

The active medium consists of an ensemble of emitters, which give rise to a band structure of energy levels.

In this case, the spontaneous emission rate into the lasing mode reads

$$r_{\text{sp}_0} = \int \int \bar{r}_{\text{sp}_0}(\mathbf{r}_e, E_{21}) \rho_{\text{elec}}(E_{21}) f_e(E_2) f_h(E_1) dE_{21} d^3\mathbf{r}_e \quad (9)$$

Here,  $\rho_{\text{elec}}(E_{21})$  is the reduced **electronic density of states** (DOS) [19, 20], which represents the density of electron-hole transitions (electronic states) per unit transition energy and per unit active region volume. The electronic DOS reflects the **inhomogeneous broadening** of the transition energy,  $E_{21} = E_2 - E_1$ , as determined by the band structure of the active medium. Here,  $E_2$ , is the energy of an electron in the conduction band, while  $E_1$  is the energy of a hole in the valence band. Both  $E_2$  and  $E_1$  are uniquely determined by  $E_{21}$ , due to conservation of energy and momentum [19, 20].

For a spontaneous emission event to happen, an electron-hole pair should be present. Hence, the product of the electron occupation probability,  $f_e(E_2)$ , and hole occupation probability,  $f_h(E_1)$ , appears in Eq. 9. Since the intraband dynamics is neglected, the occupation probabilities are Fermi-Dirac distributions. Implicitly, both probabilities were assumed to be unitary in Eq. 3. Furthermore, we note that diffusion effects are expected to even out the distribution of carriers throughout the active region. Therefore, the occupation probabilities do not depend on space. Finally, we note that the integration with respect to the emitter position,  $\mathbf{r}_e$ , is over the physical volume of the active region,  $V_{\text{act}}$ , where the emitters are spatially distributed.

By using the expression of the vacuum field, Eq. 9 becomes

$$r_{\text{sp}_0} = \frac{\hbar\omega_c}{2\epsilon_0 n_{\text{act}}^2} \Gamma \int \bar{r}_{\text{sp}_0}(E_{21}) \rho_{\text{elec}}(E_{21}) f_e(E_2) f_h(E_1) dE_{21} \quad (10)$$

where the optical confinement factor,  $\Gamma$ , reads

$$\Gamma = \frac{\int_{V_{\text{act}}} \epsilon_0 n_{\text{act}}^2 |\hat{\mathbf{d}}_e \cdot \mathbf{E}(\mathbf{r}_e)|^2 d^3\mathbf{r}_e}{\int_V \epsilon_0 n^2(\mathbf{r}) |\mathbf{E}(\mathbf{r})|^2 d^3\mathbf{r}} \quad (11)$$

Here, the active region refractive index,  $n_{\text{act}}$ , is the refractive index at the emitter position, assumed to be uniform over the active region volume. The orientation of the dipole at position  $\mathbf{r}_e$  is formally retained in Eq. 11. In practice, we may assume  $|\hat{\mathbf{d}}_e \cdot \mathbf{E}(\mathbf{r}_e)|^2 \approx |\mathbf{E}(\mathbf{r}_e)|^2$  and account for any non-perfect alignment between electric field and dipoles via an effective reduction of the amplitude of the dipole moment. For QW active media, this reduction depends on the polarization of the electric field, owing to the particular symmetries of the conduction and valence band Bloch functions [20].

With these considerations in mind, Eq. 11 is the usual expression [19] for the optical confinement factor of

semiconductor lasers theory. We note that the amplitude of the dipole moment,  $d_e$ , in Eq. 10 is formally embedded into  $\tilde{r}_{\text{sp}_0}(E_{21})$ , but its dependence on the transition energy can be often neglected [20]. The connection with the transition matrix element,  $|M_T|^2$ , is given by  $d_e^2 = q^2|M_T|^2/(m_0\omega_c)^2$  [20], where  $m_0$  is the vacuum electron mass.

In general, Eq. 10 cannot be further simplified and it is necessary to proceed numerically. In particular, the occupation probabilities are nonlinear functions of the injection level via the quasi-Fermi levels of electrons and holes. The standard approach requires the active region to be charge neutral, implying that the total number of electrons and holes has to be the same. Thus, both quasi-Fermi levels are linked to a given number of carriers, with a relation depending on the type of active material (bulk, quantum well, etc.) [19, 20]. At a given number of carriers, the quasi-Fermi levels are found and one needs to solve the integral in Eq. 10 with respect to the transition energy. By iterating this procedure, the spontaneous emission rate into the lasing mode is found as a function of the number of carriers.

We also note that by proper modification of Eq. 10 [21–23] and applying the same procedure, one may find the stimulated emission rate and *total* spontaneous emission rate. Then, the rate equations of photons and carriers may be solved in a purely numerical fashion [21–23].

Here, we pursue a more straightforward strategy and assume a *linear* dependence of spontaneous and stimulated emission on the number of carriers. The approximation is the simplest, but widely employed for both QW [24–26] and QD [27, 28] active media, and enables analytical considerations. To single out the spontaneous emission rate per emitter,  $\gamma_r$ , from Eq. 10, we assume the occupation probabilities to be unitary, corresponding to the ideal scenario of full inversion. Under these conditions, the spontaneous emission rate into the lasing mode equals  $\gamma_r n_0$ , with  $n_0$  being the total number of carriers.

We note that the linear approximation would not hold at injection levels high enough to reach full inversion and that, in practice, the onset of lasing and other phenomena, such as temperature increase, would preclude the full inversion. Therefore, this approach should be interpreted as an extrapolation procedure.

We start by considering a QD active medium with negligible inhomogeneous broadening. In this case, the electronic DOS reads  $\rho_{\text{elec}}(E_{21}) = (2n_{\text{QD}}/V_{\text{act}})\delta(E_{21} - E_s)$  [22], where  $n_{\text{QD}}$  is the number of QDs,  $V_{\text{act}}$  is the total volume of the QDs and  $E_s$  is the energy of the ground state transition. Higher-order transitions are neglected. The factor of 2 takes into account the spin degeneracy, implying  $n_0 = 2n_{\text{QD}}$ . By requiring  $r_{\text{sp}_0} =$

$\gamma_r n_0$ , we find

$$\gamma_r = \frac{2d_e^2}{\hbar\epsilon_0 n_{\text{act}}^2} \frac{\omega_c}{\gamma_2} \frac{\Gamma}{V_{\text{act}}} \quad (12)$$

For simplicity, we have assumed the ground state transition of the QDs to be in resonance with the lasing mode. Any detuning would amount to quantitative, but not qualitative changes. Furthermore, consistently with Eq. 8, we have considered the good-cavity limit. Importantly, Eq. 12 shows that  $\gamma_r$  scales with an *effective* mode volume,  $V_{\text{eff}} = V_{\text{act}}/\Gamma$ .

In practice, the epitaxial semiconductor growth process leads to unavoidable variations in the physical size of the QDs and the formation of a wetting layer [29]. By neglecting all energy transitions higher than the ground state, the electronic DOS is usually modeled by a Gaussian distribution [20, 22], with an average ground state energy,  $E_s$ , and a standard deviation,  $\sigma$ . Hence, the integration over the transition energies reduces to a convolution between a Gaussian distribution and a Lorentzian function, reflecting inhomogeneous and homogeneous broadening, respectively.

Unfortunately, this convolution can only be computed numerically. However, it is easy to realize that the inhomogeneous broadening would effectively increase the dephasing rate,  $\gamma_2$ , in Eq. 12. One may approximate the Gaussian distribution with a Lorentzian function having the same full width at half-maximum,  $2\sigma\sqrt{2\ln(2)}$ . By assuming, as done above,  $E_s = \hbar\omega_c$ , one would find

$$\gamma_r = \frac{2d_e^2}{\hbar\epsilon_0 n_{\text{act}}^2} \frac{\omega_c}{(\gamma_2 + 2\sigma\sqrt{2\ln(2)}/\hbar)} \frac{\Gamma}{V_{\text{act}}} \quad (13)$$

Hence, the inhomogeneous broadening would amount to quantitative, but not qualitative changes in the expression of  $\gamma_r$ .

Finally, we consider a QW active medium. In this case, the reduced electronic DOS is a staircase function [20], reflecting the presence of multiple subbands. Hence, the integration over the transition energies generally depends in a nontrivial manner on the energy difference between the subbands edges and the relative position of the lasing mode frequency. However, we may attempt a rough estimate by assuming the lasing mode to be in resonance with the ground state and neglecting higher-order subbands. Hence, the reduced electronic DOS reads  $\rho_{\text{elec}} = m_r/(d_{\text{QW}}\pi\hbar^2)$ , where  $m_r$  is the reduced effective mass and  $d_{\text{QW}}$  the thickness of any of the QW layers.

By using Eq. 10 under the assumption of full inversion and good-cavity limit, we find

$$r_{\text{sp}_0} = \gamma_r n_0 = \left( \frac{2d_e^2}{\hbar\epsilon_0 n_{\text{act}}^2} \frac{\omega_c}{\gamma_2} \frac{\Gamma}{V_{\text{act}}} \right) \left( \frac{m_r \gamma_2 V_{\text{act}}}{4\hbar d_{\text{QW}}} \right) \quad (14)$$

from which we may identify an effective number of emitters,  $n_0 = (m_r \gamma_2 V_{\text{act}})/(4\hbar d_{\text{QW}})$ , and an expression for

$\gamma_r$  formally identical to Eq. 12. The transparency carrier density corresponding to the effective number of emitters would be  $N_{tr} = n_0/(2V_{act})$ , which is not far from typical values [20] reported in the literature. Here,  $V_{act}$  is the volume including all the QW layers.

In conclusion, the spontaneous emission rate per emitter,  $\gamma_r$ , is given by Eq. 12 for an extended active medium. Consistently with the conventional theory of semiconductor lasers [19, 20] and previous works on nanolasers [22, 23], we find  $\gamma_r$  to be inversely proportional to an effective mode volume. This mode volume is defined by the ratio between the physical volume of the active region,  $V_{act}$ , and the optical confinement factor,  $\Gamma$ , which is the fraction of electric energy stored within  $V_{act}$ . In the case of a QD active medium,  $V_{act}$  is the total volume of the QDs, that is the sum of the volumes of every single dot.

We note that the relation between  $\gamma_r$  and the differential gain [20],  $g_N$ , is

$$\gamma_r = \frac{v_g g_N}{2V_{eff}} \quad (15)$$

where  $v_g$  is a group velocity reflecting material, but not structural dispersion [30].

## II. PHOTON VARIANCE FROM THE LANGEVIN APPROACH

From a small-signal analysis of the rate equations in the main text, Eq. 5a and Eq. 5b, with added Langevin

noise forces [20], we compute the fluctuation of the photon number around the average. From this fluctuation, we subsequently compute the power spectral density of the photon number [20]. By integrating this spectral density over all frequencies, we obtain the variance of the photon number [30]

$$\langle \Delta n_p^2 \rangle = \frac{1}{\gamma} \left[ \left( 1 + \frac{\Gamma_{ee}^2}{\omega_R^2} \right) D_{pp} + \frac{\Gamma_{pe}^2}{\omega_R^2} D_{ee} + \frac{2\Gamma_{pe}\Gamma_{ee}}{\omega_R^2} D_{pe} \right] \quad (16)$$

Here,  $\Gamma_{ee} = \gamma_p + \gamma_t + 2\gamma_r n_p$ ,  $\Gamma_{ep} = \gamma_r(2n_e - n_0)$ ,  $\Gamma_{pe} = \gamma_r(2n_p + 1)$  and  $\Gamma_{pp} = \gamma_c - \gamma_r(2n_e - n_0)$  are the small-signal coefficients, with  $n_e$  and  $n_p$  being the average number of carriers and photons, respectively. The damping rate,  $\gamma$ , and the square,  $\omega_R^2$ , of the relaxation resonance frequency read  $\gamma = \Gamma_{ee} + \Gamma_{pp}$  and  $\omega_R^2 = \Gamma_{ee}\Gamma_{pp} + \Gamma_{pe}\Gamma_{ep}$ , respectively. We note that the small-signal coefficient  $\gamma_{ij}$  determines how fast carriers ( $i=e$ ) and photons ( $i=p$ ) respond to the variation in the number of carriers ( $j=e$ ) and photons ( $j=p$ ).

The Langevin noise force on the number of carriers,  $F_e(t)$ , and photons,  $F_p(t)$ , have auto-correlations given by  $\langle F_e(t)F_e(t-\tau) \rangle = 2D_{ee}\delta(\tau)$  and  $\langle F_p(t)F_p(t-\tau) \rangle = 2D_{pp}\delta(\tau)$ , respectively, with  $2D_{ee} = \gamma_p(n_0 - n_e) + \gamma_t n_e + \gamma_r n_0 n_p$  and  $2D_{pp} = \gamma_c n_p + \gamma_r n_e + \gamma_r n_0 n_p$ . The cross-correlation, instead, is  $\langle F_p(t)F_e(t-\tau) \rangle = 2D_{pe}\delta(\tau)$ , with  $2D_{pe} = -\gamma_r n_0 n_p - \gamma_r n_e$ .

- 
- [1] Y. Xu, R. K. Lee, and A. Yariv, Phys. Rev. A **61**, 033807 (2000).
  - [2] J.-M. Gérard, "Solid-state cavity-quantum electrodynamics with self-assembled quantum dots," in *Single Quantum Dots: Fundamentals, Applications, and New Concepts* (Springer Berlin Heidelberg, Berlin, Heidelberg, 2003) pp. 269–314.
  - [3] L. Novotny and B. Hecht, *Principles of Nano-Optics* (Cambridge University Press, 2006).
  - [4] R. K. Chang and A. J. Campillo, *Optical processes in microcavities* (London, 1996).
  - [5] A. W. Snyder and J. D. Love, *Optical Waveguide Theory* (Springer New York, NY, 1983).
  - [6] P. T. Kristensen, R.-C. Ge, and S. Hughes, Phys. Rev. A **92**, 053810 (2015).
  - [7] E. A. Muljarov and W. Langbein, Phys. Rev. A **96**, 017801 (2017).
  - [8] P. T. Kristensen, R.-C. Ge, and S. Hughes, Phys. Rev. A **96**, 017802 (2017).
  - [9] P. T. Kristensen, C. V. Vlack, and S. Hughes, Opt. Lett. **37**, 1649 (2012).
  - [10] C. Sauvan, J. P. Hugonin, I. S. Maksymov, and P. Lalanne, Phys. Rev. Lett. **110**, 237401 (2013).
  - [11] P. Lalanne, W. Yan, K. Vynck, C. Sauvan, and J.-P. Hugonin, Laser & Photonics Reviews **12**, 1700113 (2018).
  - [12] P. T. Kristensen, K. Herrmann, F. Intravaia, and K. Busch, Adv. Opt. Photon. **12**, 612 (2020).
  - [13] J. D. Joannopoulos, S. G. Johnson, J. N. Winn, and R. D. Meade, *Photonic Crystals: Molding the Flow of Light - Second Edition*, rev - revised, 2 ed. (Princeton University Press, 2008).
  - [14] R. El-Ganainy, K. G. Makris, M. Khajavikhan, Z. H. Musslimani, S. Rotter, and D. N. Christodoulides, Nature Physics **14**, 11 (2018).
  - [15] R.-M. Ma, R. F. Oulton, V. J. Sorger, and X. Zhang, Laser & Photonics Reviews **7**, 1 (2013).
  - [16] S. Gwo and C.-K. Shih, Reports on Progress in Physics **79**, 086501 (2016).
  - [17] P. Borri, W. Langbein, J. M. Hvam, F. Heinrichsdorff, M.-H. Mao, and D. Bimberg, Applied Physics Letters **76**, 1380 (2000).
  - [18] E. Purcell, Phys. Rev. **69**, 674 (1946).
  - [19] T. Suhara, *Semiconductor Laser Fundamentals*, 1st ed.

- (CRC Press, 2004).
- [20] L. A. Coldren, S. W. Corzine, and M. Mašanović, *Diode Lasers and Photonic Integrated Circuits*, 2nd ed. (John Wiley & Sons, Inc., 2012).
  - [21] N. Gregersen, T. Suhr, M. Lorke, and J. Mørk, *Applied Physics Letters* **100**, 131107 (2012).
  - [22] M. Lorke, T. Suhr, N. Gregersen, and J. Mørk, *Phys. Rev. B* **87**, 205310 (2013).
  - [23] B. Romeira and A. Fiore, *IEEE Journal of Quantum Electronics* **54**, 1 (2018).
  - [24] S. Matsuo, T. Sato, K. Takeda, A. Shinya, K. Nozaki, H. Taniyama, M. Notomi, K. Hasebe, and T. Kakitsuka, *IEEE Journal of Selected Topics in Quantum Electronics* **19**, 4900311 (2013).
  - [25] N. Takemura, M. Takiguchi, E. Kuramochi, A. Shinya, T. Sato, K. Takeda, S. Matsuo, and M. Notomi, *Phys. Rev. A* **99**, 053820 (2019).
  - [26] E. Dimopoulos, A. Sakanas, A. Marchevsky, M. Xiong, Y. Yu, E. Semenova, J. Mørk, and K. Yvind, *Laser & Photonics Reviews* **n/a**, 2200109.
  - [27] Y. Ota, M. Kakuda, K. Watanabe, S. Iwamoto, and Y. Arakawa, *Opt. Express* **25**, 19981 (2017).
  - [28] A. Kaganskiy, S. Kreinberg, X. Porte, and S. Reitzenstein, *Optica* **6**, 404 (2019).
  - [29] A. Sobiesierski and P. Snowton (Elsevier, Amsterdam, 2011) pp. 353–384.
  - [30] J. Mørk and G. L. Lippi, *Applied Physics Letters* **112**, 141103 (2018).
